# Supplementary material for: Transformers are Provably Optimal In-context Estimators for Wireless Communications
Source: arXiv:2311.00226 source file (2025-03-11)
Supplement: Supplementary file 1 [file appendix-BPSK.tex]

\section{Appendix for Binary Estimation}
\label{sec:appendix}

\emph{Proof of Lemma \ref{lem:opt-MMSE}}. Let $p(\vy \mid \vh)$ denote the conditional density of $\vy$ for a given $\vh$. Let $p_{\bepsilon}$ denote the density of $\bepsilon$. Since $x \sim \cU\{\pm 1\}$ and $\tanh(z) = \frac{1-e^{-2z}}{1+e^{-2z}}$, we can compute
\begin{align*}
    \hat{x}_{\rm MMSE}(\vy, \vh; \bSigma_{\bepsilon}) &= \bE_{x, \bepsilon}[x \mid \vy, \vh]  = \bP(x = 1 \mid \vy, \vh) - \bP(x = -1 \mid \vy, \vh) \\
    &= \frac{1}{p(\vy \mid \vh)}(\bP(x = 1) p(\vy \mid \vh, x = 1) - \bP(x = -1) p(\vy \mid \vh, x = -1)) \\
    &=\frac{\bP(x = 1) p(\vy \mid \vh, x = 1) - \bP(x = -1) p(\vy \mid \vh, x = -1)}{\bP(x = 1) p(\vy \mid \vh, x = 1) + \bP(x = -1) p(\vy \mid \vh, x = -1)} \\
    &= \frac{ p(\vy \mid \vh, x = 1) - p(\vy \mid \vh, x = 1)}{p(\vy \mid \vh, x = 1) + p(\vy \mid \vh, x = 1)} = \frac{ p_{\bepsilon}(\vy-\vh) - p_{\bepsilon}(\vy+\vh)}{p_{\bepsilon}(\vy-\vh) + p_{\bepsilon}(\vy+\vh)} \\
    &= \frac{\exp(-\frac{1}{2}(\vy-\vh)^T \bSigma_{\bepsilon}^{-1}(\vy-\vh))-\exp(-\frac{1}{2}(\vy+\vh)^T \bSigma_{\bepsilon}^{-1}(\vy+\vh))}{\exp(-\frac{1}{2}(\vy-\vh)^T \bSigma_{\bepsilon}^{-1}(\vy-\vh))+\exp(-\frac{1}{2}(\vy+\vh)^T \bSigma_{\bepsilon}^{-1}(\vy+\vh))} \\
    &= \frac{1-\exp(-2 \vy^T \bSigma_{\bepsilon}^{-1} \vh)}{1+\exp(-2 \vy^T \bSigma_{\bepsilon}^{-1} \vh)} = \tanh(\vy^T \bSigma_{\bepsilon}^{-1} \vh).
\end{align*}

\emph{Proof of Lemma \ref{lem:convergence-SA}}. Let the prompt correspond to $\vh$, and thus $\vy_i = \vh x_i + \bepsilon_i$, $\vy = \vh x + \bepsilon$. Therefore, the expression for the output of the transformer is given by
\begin{align*}
    &T_n^{\rm SA}(\vy, \{\vy_i\}_1^n, \{x_i\}_1^n;\mW ) =
    \frac{\sum_{i=1}^n x_i \exp(\vy^T \mW \vy_i)}{\exp(\vy^T \mW \vy) + \sum_{i=1}^n \exp(\vy^T \mW \vy_i)} \\
    &\hspace{15pt} = x \cdot \frac{e^{x\vy^T \mW \vh} \frac{\abs{I_n^+}}{n} \frac{1}{\abs{I_n^+}}\sum_{i\in I_n^+} e^{\vy^T \mW \bepsilon_i} - e^{-x\vy^T \mW \vh} \frac{\abs{I_n^-}}{n} \frac{1}{\abs{I_n^-}}\sum_{i\in I_n^-} e^{\vy^T \mW \bepsilon_i}}{\frac{1}{n} e^{\vy^T \mW \vy} + e^{x\vy^T \mW \vh} \frac{\abs{I_n^+}}{n} \frac{1}{\abs{I_n^+}}\sum_{i\in I_n^+} e^{\vy^T \mW \bepsilon_i} + e^{-x\vy^T \mW \vh} \frac{\abs{I_n^-}}{n} \frac{1}{\abs{I_n^-}}\sum_{i\in I_n^-} e^{\vy^T \mW \bepsilon_i}},
\end{align*}
where $I_n^+ \triangleq \{i\in [n]: x_i = x\}$ and $I_n^- \triangleq \{i\in [n]: x_i = -x\}$. By the strong law of large numbers, we have a.s. that
\begin{align*}
    \lim_{n\to \infty} \frac{\abs{I_n^+}}{n} &= \lim_{n\to \infty} \frac{1}{n}\sum_{i=1}^n \mathbf{1}_{\{x_i = x\}} = \bE[\mathbf{1}_{\{x_1 = x\}}] = \bP(x_1 = x) = \frac{1}{2} = \bP(x_1 = -x) = \lim_{n\to \infty} \frac{\abs{I_n^-}}{n}
\end{align*}
In particular, this implies that $\abs{I_n^+}, \abs{I_n^-} \to \infty$ a.s. Therefore, by another application of the strong law of large numbers, we obtain a.s.
\begin{align*}
    \lim_{n\to \infty} \frac{1}{\abs{I_n^+}} \sum_{i\in I_n^+} e^{\vy^T \mW \bepsilon_i} = \bE_{\bepsilon}[e^{\vy^T \mW \bepsilon}] = \lim_{n\to \infty} \frac{1}{\abs{I_n^-}} \sum_{i\in I_n^-} e^{\vy^T \mW \bepsilon_i},
\end{align*}
and note that this is a strictly positive finite quantity. Thus, by cancellation we obtain that a.s.
\begin{align*}
    \lim_{n\to \infty} T_n^{\rm SA}(\vy, \{\vy_i\}_1^n, \{x_i\}_1^n; \mW) &= x \cdot \frac{e^{x\vy^T \mW \vh}-e^{-x\vy^T \mW \vh}}{e^{x\vy^T \mW \vh}+e^{-x\vy^T \mW \vh}}\\
    &= \frac{e^{\vy^T \mW \vh}-e^{-\vy^T\mW \vh}}{e^{\vy^T \mW \vh}+e^{-\vy^T\mW \vh}} = \tanh(\vy^T \mW \vh).
\end{align*}

\emph{Proof of Theorem \ref{thm:global-min}}. 
From Lemma \ref{lem:convergence-SA}, we get 
\begin{align*}
    \lim_{n\to \infty} T_n^{\rm SA}(\vy, \{\vy_i\}_1^n, \{x_i\}_1^n; \mW) = \hat{x}_{\rm MMSE}(\vy, \vh;\mW)~{\rm a.s.}
\end{align*}
Since
\begin{align*}
    \abs{T_n^{\rm SA}(\vy, \{\vy_i\}_1^n, \{x_i\}_1^n; \mW)} &= \Big| \frac{\sum_{i=1}^n x_i \exp(\vy^T \mW \vy_i)}{\exp(\vy^T \mW \vy) + \sum_{i=1}^n \exp(\vy^T \mW \vy_i)} \Big| \\
    &\le \frac{\sum_{i=1}^n \abs{x_i} \exp(\vy^T \mW \vy_i)}{\sum_{i=1}^n \exp(\vy^T \mW \vy_i)} = 1,
\end{align*}
we have $\forall \mW \in \bR^{d\times d}, \forall n\ge 0$, $0\le g_n(\mW) \triangleq (T_n^{\rm SA}(\vy, \{\vy_i\}_1^n, \{x_i\}_1^n; \mW)-x)^2 \le 4$. Thus, $\{g_n(\mW)\}_1^\infty$ are bounded, integrable random variables. Therefore, using the bounded convergence theorem (BCT), we get
\begin{align*}
    \cL(\mW; \mu_\vh, \bSigma_{\bepsilon}) &\triangleq \limsup_{n\to \infty}\bE[g_n(\mW)] = \bE[\limsup_{n\to\infty} g_n(\mW)] \\
    &= \bE[(\limsup_{n\to\infty}T_n^{\rm SA}(\vy, \{\vy_i\}_1^n, \{x_i\}_1^n; \mW) -x)^2] \\
    &=\bE_{\vh, x,\bepsilon}[(\hat{x}_{\rm MMSE}(\vy, \vh;\mW)-x)^2] \\
    &= \bE_{\mu_\vh}[\bE_{x,\bepsilon}[(\hat{x}_{\rm MMSE}(\vy, \vh;\mW)-x)^2\mid \vh]] \triangleq \bE_{\mu_\vh}[\delta_\vh(\mW; \bSigma_{\bepsilon})],
\end{align*}
where $\delta_\vh(\mW; \bSigma_{\bepsilon}) \triangleq \bE_{x,\bepsilon}[(\hat{x}_{\rm MMSE}(\vy, \vh;\mW)-x)^2 \mid \vh]$, where $\mu_\vh$ is the distribution of $\vh$ across the prompts during training.

Let $\vh \in \bR^d$ is the channel corresponding to a prompt in the training. For $n\ge 0$, let $\cX^n_\vh \triangleq \{f \in L^2: f ~{\rm is}~\sigma(\vy, \{\vy_i\}_1^n, \{x_i\}_1^n, \vh){\rm-measurable}\}$, where the random variables satisfy $\vy = \vh x + \bepsilon, \vy_i = \vh x_i + \bepsilon_i$ for the given $\vh\in\bR^d$. Consider the minimization problem $\min_{\hat{x}_n \in \cX^n_\vh} \bE[(\hat{x}_n-x)^2]$, where the expectation is over the prompt characterizing the set $\cX_\vh^n$. Then, the minimizer is the conditional expectation which by Lemma \ref{lem:opt-MMSE} is given as
\begin{align*}
    \hat{x}^*(\vy, \{\vx_i\}_1^{n}, \{x_i\}_1^n, \vh) &= \bE[x \mid \vy, \{\vy_i\}_1^{n}, \{x_i\}_1^n, \vh] = \bE_{x, \bepsilon}[x \mid \vy, \vh] \\
    &= \tanh(\vy^T \bSigma_{\bepsilon}^{-1}\vh) = \hat{x}_{\rm MMSE}(\vy, \vh; \bSigma_{\bepsilon}),
\end{align*}
and the minimum value is $\bE_{x,\bepsilon}[(\hat{x}_{\rm MMSE}(\vy, \vh; \bSigma_{\bepsilon})-x)^2\mid \vh] = \delta_\vh(\bSigma_{\bepsilon}^{-1}; \bSigma_{\bepsilon})$. Thus, we just showed that $\forall n \ge 0,\forall \hat{x}_n \in \cX^n_\vh$, we have $\bE[(\hat{x}_n-x)^2 \mid \vh] \ge \delta_\vh(\bSigma_{\bepsilon}^{-1}; \bSigma_{\bepsilon})$. In particular, for any fixed $\vh$ in the training, $\forall \mW \in \bR^{d\times d}$, $\forall n \ge 0$ since $T_n^{\rm SA}(\cdot ;\mW) \in \cX^n_\vh$, we have $\bE_{x, \bepsilon}[(T_n^{\rm SA}(\cdot; \mW)-x)^2 \mid \vh] \ge \delta_\vh(\bSigma_{\bepsilon}^{-1}; \bSigma_{\bepsilon})$. Taking expectations on both sides with respect to the distribution $\mu_\vh$ of $\vh$ during pre-training, we get that $\cL_n(\mW; \mu_\vh, \bSigma_{\bepsilon}) \ge \bE_{\mu_\vh}[\delta_\vh(\bSigma_{\bepsilon}^{-1}; \bSigma_{\bepsilon})]$. Finally, taking limit on the left hand side we get that for any $\mu_\vh$ and $\mW \in \bR^{d\times d}$, 
\begin{align*}
    \cL(\mW; \mu_\vh, \bSigma_{\bepsilon}) = \limsup_{n\to \infty} \cL_n(\mW; \mu_\vh, \bSigma_{\bepsilon}) \ge \bE_{\mu_\vh}[\delta_\vh(\bSigma_{\bepsilon}^{-1}; \bSigma_{\bepsilon})] = \cL(\bSigma_{\bepsilon}^{-1}; \mu_\vh, \bSigma_{\bepsilon}),
\end{align*}
whence $\mW^* \triangleq \bSigma_{\bepsilon}^{-1}$ is the global minimizer of $\cL(\cdot; \mu_\vh, \bSigma_{\bepsilon})$.
