# Supplementary material for: Transformers are Provably Optimal In-context Estimators for Wireless Communications
Source: arXiv:2311.00226 source file (2025-03-11)
Supplement: Supplementary file 2 [file appendix-PSK.tex]

\section{Appendix for Theoretical Results}

\label{sec:appendix-finite-estimation}

\emph{Proof of Lemma \ref{lem:opt-MMSE-PSK}}. Let $p(\vy \mid \mH)$ denote the conditional density of $\vy$ for a given $\mH$, and let $\bP(\vx \mid \vy , \mH)$ denote the posterior probability of $\vx \in \cX$ given $\vy , \mH$. Let $p_{\vz}$ denote the density of $\vz$, which is the normal density with mean $\0 \in \bR^d$ and covariance $\bSigma_z = \frac{1}{2} \begin{bmatrix}
    \tilde{\bSigma}_z & \0 \\
    \0 & \tilde{\bSigma}_z
\end{bmatrix} \in \bR^{2d\times 2d}$. Note that $\bSigma_z^{-1} = 2 \begin{bmatrix}
    \tilde{\bSigma}_z^{-1} & \0 \\
    \0& \tilde{\bSigma}_z^{-1}
\end{bmatrix}$. Since $\vx, \mH$ are independent, $\bP(\vx \mid \mH) = \bP(\vx)$.
We can therefore write
\begin{align*}
    &\hat{\vx}_{\rm MMSE}(\vy, \mH; \tilde{\bSigma}_z, \bP_x) = \bE[\vx \mid \vy, \vh] = \sum_{\vx \in \cX} \vx \bP(\vx \mid \vy, \mH) \\
    &= \sum_{\vx \in \cX} \vx \frac{\bP(\vx \mid \mH) p( \vy \mid \vx, \mH)}{p(\vy \mid \mH)} = \frac{\sum_{\vx \in \cX} \vx \bP(\vx \mid \mH) p( \vy \mid \vx, \mH)}{\sum_{\vx \in \cX}\bP(\vx \mid \mH) p( \vy \mid \vx, \mH)} = \frac{\sum_{\vx \in \cX} \vx \bP(\vx) p( \vy \mid \vx, \mH)}{\sum_{\vx \in \cX} \bP(\vx) p( \vy \mid \vx, \mH)}.
\end{align*}
Now, we can first compute 
\begin{align*}
     p( \vy \mid \vx, \mH) = p_{\vz}(\vy-\mH\vx) 
     &\propto \exp \left( -\frac{1}{2} (\vy-\mH\vx)^T \bSigma_z^{-1} (\vy - \mH\vx) \right) \\
     &=\exp \left( \vy^T\bSigma_z^{-1}\mH\vx-\frac{1}{2}\vy^T \bSigma_z^{-1}\vy-\frac{1}{2}\vx^T\mH^T \bSigma_z^{-1} \mH\vx \right).
\end{align*}
% Since $\vx \in \cX$ iff $-\vx \in \cX$, we can construct a disjoint partition of $\cX$ to be $\cX^+, \cX^-$ such that $-\cX^+ = \cX^-$. Then
% \begin{align*}
%     &\sum_{\vx \in \cX} \vx p (\vy \mid \vx, \mH) = \sum_{\vx \in \cX^{+}} \vx (p(\vy \mid \vx, \mH) -p(\vy \mid -\vx, \mH)) \\
%     &\propto \exp(-\frac{1}{2} \vy^T \bSigma_z^{-1}\vy) \sum_{\vx \in \cX^+} \vx \exp(-\frac{1}{2}\vx^T\mH^T \bSigma_z^{-1} \mH\vx)(\exp(\vy^T\bSigma_z^{-1}\mH\vx)-\exp(-\vy^T\bSigma_z^{-1}\mH\vx)).
% \end{align*}
Then, we simplify denoting $\vh_I \triangleq \operatorname{Re}(\tilde{\vh}), \vh_Q \triangleq \operatorname{Im}(\tilde{\vh})$
\begin{align*}
    \frac{1}{2} \mH^T \bSigma_z^{-1} \mH &=  \begin{bmatrix}
        \vh_I^T & \vh_Q^T \\
        -\vh_Q^T & \vh_I^T
    \end{bmatrix}
    \begin{bmatrix}
    \tilde{\bSigma}_z^{-1} & \0 \\
    \0& \tilde{\bSigma}_z^{-1}
\end{bmatrix}
 \begin{bmatrix}
        \vh_I & -\vh_Q \\
        \vh_Q & \vh_I
    \end{bmatrix} \\
    &=
    \begin{bmatrix}
        \vh_I^T & \vh_Q^T \\
        -\vh_Q^T & \vh_I^T
    \end{bmatrix}
    \begin{bmatrix}
        \tilde{\bSigma}_z^{-1}\vh_I & -\tilde{\bSigma}_z^{-1}\vh_Q \\
        \tilde{\bSigma}_z^{-1}\vh_Q & \tilde{\bSigma}_z^{-1}\vh_I
    \end{bmatrix}\\
    &=
    \begin{bmatrix}
       \vh_I^T \tilde{\bSigma}_z^{-1} \vh_I + \vh_Q^T \tilde{\bSigma}_z^{-1} \vh_Q & 0 \\
       0 & \vh_I^T \tilde{\bSigma}_z^{-1} \vh_I + \vh_Q^T \tilde{\bSigma}_z^{-1} \vh_Q
    \end{bmatrix}
    = \gamma_{z, \vh} \mI_2,
\end{align*}
where $\gamma_{z, \vh} \triangleq \vh_I^T \tilde{\bSigma}_z^{-1} \vh_I + \vh_Q^T \tilde{\bSigma}_z^{-1} \vh_Q$ denotes the instantaneous signal to noise ratio (SNR). Thus, the expression for $\hat{\vx}_{\rm MMSE}(\vy, \vh; \tilde{\bSigma}_z, \cX)$ using $\vx^T \vx = 1$ for $\vx \in \cX$ is given by
\begin{align*}
    \hat{\vx}_{\rm MMSE}(\vy, \vh; \bSigma_z, \bP_x) &= \frac{\exp(-\frac{1}{2} \vy^T \bSigma_z^{-1}\vy)\sum_{\vx \in \cX} \vx\bP(\vx) \exp(\vy^T \bSigma_z^{-1} \mH \vx) \exp(-\gamma_{z, \vh}\vx^T\vx)}{\exp(-\frac{1}{2} \vy^T \bSigma_z^{-1}\vy)\sum_{\vx \in \cX} \bP(\vx) \exp(\vy^T \bSigma_z^{-1} \mH \vx) \exp(-\gamma_{z, \vh}\vx^T\vx)} \\
    &= \frac{\sum_{\vx \in \cX}\vx \bP_x(\vx)\exp(\vy^T \bSigma_z^{-1} \mH \vx)}{\sum_{\vx \in \cX} \bP_x(\vx)\exp(\vy^T \bSigma_z^{-1} \mH \vx)}.
\end{align*}

\emph{Proof of Lemma \ref{lem:convergence-SA-PSK}}. Let the prompt $\mU_{n+1}$ correspond to $\vh$, and thus $\vy = \mH \vx + \vz$, $\vy_i = \mH \vx_i + \vz_i$, for $i\in[n]$. For $\vx \in \cX$, denoting $\cI_\vx^n \triangleq \{i\in [n]: \vx_i = \vx\}$, the quantity $\hat{\vx}^{\rm SA}_{n}(\mU_{n+1}; \mW)$ is given by
\begin{align*}
    &\frac{\sum_{i=1}^n \vx_i \exp(\vy^T \mW \vy_i)}{\exp(\vy^T \mW \vy) + \sum_{i=1}^n \exp(\vy^T \mW \vy_i)}  = \frac{\sum_{\vx \in \cX} \sum_{i\in \cI_{\vx}^n} \vx_i \exp(\vy^T \mW \vy_i)}{\exp(\vy^T \mW \vy)  + \sum_{\vx \in \cX} \sum_{i\in \cI_{\vx}^n} \exp(\vy^T \mW \vy_i)} \\
    &\hspace{40pt} = \frac{\sum_{\vx \in \cX} \vx \exp(\vy^T \mW \mH \vx) \frac{\abs{\cI_\vx^n}}{n} \frac{1}{\abs{\cI_{\vx}^n}} \sum_{i\in \cI_{\vx}^n} \exp(\vy^T \mW \vz_i)}{\frac{1}{n} \exp(\vy^T \mW \vy) + \sum_{\vx \in \cX} \exp(\vy^T \mW \mH \vx) \frac{\abs{\cI_\vx^n}}{n} \frac{1}{\abs{\cI_{\vx}^n}} \sum_{i\in \cI_{\vx}^n} \exp(\vy^T \mW \vz_i)}
\end{align*}
By the strong law of large numbers, we have almost surely
\begin{align*}
    \lim_{n\to \infty} \frac{\abs{\cI_\vx^n}}{n} = \lim_{n\to \infty} \frac{1}{n}\sum_{i=1}^n \mathbf{1}_{\{\vx_i = \vx\}} = \bE[\mathbf{1}_{\{\vx_1 = \vx\}}] = \bP_x(\vx) .
\end{align*}
In particular, this implies that $\abs{\cI_{\vx}^n} \to \infty$ a.s., for all $\vx \in \cX$. Therefore, by another application of the strong law of large numbers to the (iid log-normal random variables) $\exp(\vy^T\mW \vz_i), i\in \cI_\vx^n$ of finite mean (and second moment), we obtain that almost surely
\begin{align*}
    \lim_{n\to \infty} \frac{1}{\abs{\cI_{\vx}^n} } \sum_{i\in \cI_{\vx}^n} \exp(\vy^T \mW \vz_i) = \bE_{\vz}[\exp(\vy^T \mW \vz)],
\end{align*}
and note that this is a strictly positive finite quantity. Thus, by cancellation, we obtain
\begin{align*}
    \lim_{n\to \infty} \hat{\vx}^{\rm SA}_{n}(\mU_{n+1}; \mW) &= \frac{\sum_{\vx \in \cX} \vx  \bP_x(\vx) \exp(\vy^T \mW \mH \vx)}{\sum_{\vx \in \cX}  \bP_x(\vx) \exp(\vy^T \mW \mH \vx)} ~{\rm a.s}.
\end{align*}

\emph{Proof of Theorem \ref{thm:global-min-PSK}}. 
From Lemma \ref{lem:convergence-SA-PSK}, we get 
\begin{align*}
    \lim_{n\to \infty} \hat{\vx}_n^{\rm SA}(\mU_{n+1}; \mW) = \frac{\sum_{\vx\in \cX} \vx \bP_x(\vx) \exp(\vy^T \mW \mH \vx) }{\sum_{\vx\in \cX} \bP_x(\vx) \exp(\vy^T \mW \mH\vx)} \triangleq f(\mW; \vy,\mH,\bP_x) ~{\rm a.s.}
\end{align*}
Since $\norm{\vx_i}_2 = 1$ for any $i\in[n]$, we get
\begin{align*}
    \norm{\hat{\vx}_n^{\rm SA}(\mU_{n+1}; \mW)}_2 &= \left\| \frac{\sum_{i=1}^n \vx_i \exp(\vy^T \mW \vy_i)}{\exp(\vy^T \mW \vy) + \sum_{i=1}^n \exp(\vy^T \mW \vy_i)} \right\|_2 \\
    &\le \frac{\sum_{i=1}^n \norm{\vx_i}_2 \exp(\vy^T \mW \vy_i)}{\sum_{i=1}^n \exp(\vy^T \mW \vy_i)} = 1,
\end{align*}
we have $\forall \mW \in \bR^{d\times d}, \forall n\ge 0$, $0\le g_n(\mW) \triangleq \norm{\hat{\vx}_n^{\rm SA}(\mU_{n+1}; \mW)-\vx}_2^2 \le 4$. Thus, $\{g_n(\mW)\}_1^\infty$ are bounded, integrable random variables. Therefore, using the bounded convergence theorem (BCT), we get
\begin{align*}
    \cL(\mW; \bSigma_z, \bP_x, \bP_{\Theta,h}) &\triangleq \limsup_{n\to \infty}\bE[g_n(\mW)] = \bE[\limsup_{n\to\infty} g_n(\mW)] \\
    &= \bE[\norm{\limsup_{n\to\infty}\hat{\vx}_n^{\rm SA}(\mU_{n+1}; \mW) -\vx}_2^2] \\
    &=\bE[\norm{f(\mW; \vy,\mH,\bP_x)-\vx}_2^2] \\
    &= \bE_{\theta\sim \bP_\Theta, \mH \sim P_{h\mid \theta}}[\bE[\norm{f(\mW; \vy,\mH,\bP_x)-\vx}_2^2\mid \mH]]\\
    &\triangleq \bE_{\theta\sim \bP_\Theta, \mH \sim P_{h\mid \theta}}[\delta_\mH(\mW; \bSigma_z, \bP_x)],
\end{align*}
where $\delta_\mH(\mW; \bSigma_z, \bP_x) \triangleq \bE_{\vx \sim \bP_x, \vz \sim \cN(\0, \bSigma_z)}[\norm{f(\mW; \vy,\mH,\bP_x)-\vx}_2^2\mid \mH]$, and $\bP_{\Theta, h}$ determines the distribution of $\mH$ across the prompts during training.

Let $\mH \in \bR^{2d\times 2}$ is the channel matrix corresponding to $\vh \in \bC^d$ for a prompt in the training. For $n\ge 0$, let $\cF^n_{\mH} \triangleq \{f \in L^2: f ~{\rm is}~\sigma(\vy, \{\vy_i\}_1^n, \{\vx_i\}_1^n, \mH){\rm-measurable}\}$, where the random variables satisfy $\vy = \mH \vx + \vz, \vy_i = \mH \vx_i + \vz_i$. Consider the minimization problem $\min_{\hat{\vx}_n \in \cF^n_\mH} \bE[\norm{\hat{\vx}_n-\vx}_2^2]$, where the expectation is over the prompt characterizing the set $\cF_\mH^n$. Then, the minimizer is the conditional expectation which by Lemma \ref{lem:opt-MMSE-PSK} is given as
\begin{align*}
    \hat{\vx}^*(\vy, \{\vx_i\}_1^{n}, \{\vx_i\}_1^n, \mH) &= \bE[\vx \mid \vy, \{\vy_i\}_1^{n}, \{\vx_i\}_1^n, \mH] = \bE[\vx \mid \vy, \mH]  \\
    &= \hat{\vx}_{\rm MMSE}(\vy, \mH; \bSigma_z, \bP_x) = f(\bSigma_z^{-1}; \vy, \mH, \bP_x),
\end{align*}
and the minimum is $\bE_{\vx \sim \bP_x,\vz \sim \cN(\0, \bSigma_z)}[\norm{\hat{\vx}_{\rm MMSE}(\vy, \mH; \bSigma_z, \bP_x)-\vx}_2^2\mid \mH] = \delta_\mH(\bSigma_z^{-1}; \bSigma_z, \bP_x)$. Thus, we just showed that $\forall n \ge 0,\forall \hat{\vx}_n \in \cF^n_\mH$, we have $\bE[\norm{\hat{\vx}_n-\vx}_2^2 \mid \mH] \ge \delta_\mH(\bSigma_z^{-1}; \bSigma_z, \bP_x)$. In particular, for any fixed $\mH$ in the training, $\forall \mW \in \bR^{2d\times 2d}$, $\forall n \ge 0$ since $\hat{\vx}_n^{\rm SA}(\cdot ;\mW) \in \cF^n_\mH$, we have $\bE_{\vx\sim\bP_x, \vz \sim \cN(\0, \bSigma_z)}[\norm{\hat{\vx}_n^{\rm SA}(\cdot; \mW)-\vx}_2^2 \mid \mH] \ge \delta_\mH(\bSigma_z^{-1}; \bSigma_z, \bP_x)$. Taking expectations on both sides with respect to the distribution $\bP_{\Theta, h}$ of $\mH$ during pre-training, we get that $ \cL(\mW; \bSigma_z, \bP_x, \bP_{\Theta,h}) \ge \bE_{\theta\sim \bP_\Theta, \mH \sim P_{h\mid \theta}}[\delta_\mH(\bSigma_z^{-1}; \bSigma_z,\bP_x)]$. Taking limit we get that for any $\bP_{\Theta, h}$ and $\bP_x$ on some finite set $\cX \subset \bS^2$ and $\mW \in \bR^{2d\times 2d}$, 
\begin{align*}
   \cL(\mW; \bSigma_z, \bP_x, \bP_{\Theta,h}) &= \limsup_{n\to \infty} \cL_n(\mW; \bSigma_z, \bP_x, \bP_{\Theta,h}) \\
   &\ge \bE_{\theta\sim \bP_\Theta, \mH \sim P_{h\mid \theta}}[\delta_\mH(\bSigma_z^{-1}; \bSigma_z, \bP_x)] =  \cL(\bSigma_z^{-1}; \bSigma_z, \bP_x, \bP_{\Theta,h}),
\end{align*}
whence $\mW^* \triangleq \bSigma_z^{-1}$ is the global minimizer of $ \cL(\cdot; \bSigma_z, \bP_x, \bP_{\Theta,h})$.
